# Supplementary material for: Uncertainty-Aware Adaptive Dynamics For Underwater Vehicle-Manipulator Robots
Source: arXiv:2603.06548 source file (2026-03-06)
Supplement: Supplementary file 1 [file appendix.tex]

% ---------------------------------------- Section begin -----------------------------------------------------
\vspace{-5pt}
\section{Appendix}
\label{sec:appendix}
\subsection{Hydrodynamics Informed 
 \ac{RNEA}}
 \label{appen:RNEA}
%\subsubsection*{Algorithm Details}
The algorithm starts by assuming the dynamics of the  free-floating base in the body coordinate system is available. The free-floating base can be represented by an underwater vehicle such as a \ac{ROV} or \ac{AUV}. The  dynamics of this can be modeled using Fossen's formulation for underwater vehicles \cite{9781119994138ch6}. In this work, the free-floating base has been represented as a floating joint. The body frame of the free-floating base becomes the main coordinate frame with respect to which  the entire system is represented.   %enabling the calculation of the inverse dynamics $\boldsymbol{\tau}$ of the underwater manipulation system.

\begin{algorithm}[!htb]
\caption{}%Hydrodynamics Informed RNEA}
\label{alg:hyd_rnea}
\begin{algorithmic}[1]
% \Require 
% \State $\boldsymbol{q}^n, \boldsymbol{\dot{q}}^n, \boldsymbol{\Ddot{q}}^n$ \Comment{arm joints position, velocity, acceleration}
% \State $\pi_{base}=: \{\boldsymbol{v_{base}}, \boldsymbol{a_{base}}, \boldsymbol{f_{base}^B}, \boldsymbol{{}^0X_{base}}\}$ \Comment{floating base states and corresponding body forces and moments}
% \Ensure 
% \State $\boldsymbol{\tau} = \boldsymbol{id_{rnea}}(\boldsymbol{q}^n, \boldsymbol{\dot{q}}^n, \boldsymbol{\Ddot{q}},\pi_{base})  = vertcat(\boldsymbol{\tau_{base}}, \boldsymbol{\tau_{motor}})$

\Ensure 
\For{$i=1$ to $N_B$}
    \State $[\boldsymbol{{}^iX_{\lambda(i)}}, \boldsymbol{s_i}] = joint\_model(i, q_i)$
    \If {$\lambda(i) \neq 0$}
        \State $\boldsymbol{{}^iX_{v}={}^iX_{\lambda(i)}{}^{\lambda(i)}X_0{}^0X_{v}}$
    \Else
        \State $\boldsymbol{v_0} = \boldsymbol{{}^0X_{v}}\boldsymbol{v_{v}}$ 
        \State $\boldsymbol{a_0} = \boldsymbol{{}^0X_{v}}\boldsymbol{a_{v}}$ 
    \EndIf
    \State $\boldsymbol{v_i} = \boldsymbol{{}^iX_{\lambda(i)}}\boldsymbol{v_{\lambda(i)}} \boldsymbol{+}\boldsymbol{s_i}\dot{q_i}$
    \State $\boldsymbol{a_i} = \boldsymbol{{}^iX_{\lambda(i)}}\boldsymbol{a_{\lambda(i)}} \boldsymbol{+} \boldsymbol{s_i}\Ddot{q_i} + \boldsymbol{v_i} \times \boldsymbol{s_i}\dot{q_i}$
    \State $\boldsymbol{f_i^B = I_ia_i + S(v_i)I_iv_i}$ 
    \State $\boldsymbol{f_i^H = M_{A_i}a_i + C(v_i)_{A_i}v_i + D(v_i)_iv_i -g_i(\eta)}$ 
    \State $\boldsymbol{f_i = f_i^B - f_i^H}$
\\
    \State $\boldsymbol{v^R_{i}} = \boldsymbol{{}^iX_{\lambda(i)}v_{\lambda(i)}} \boldsymbol{+} \boldsymbol{s_i}G_i\dot{q_i}$ 
    \State $\boldsymbol{a^R_{i} ={}^iX_{\lambda(i)}a_{\lambda(i)} + s_i}G_i\Ddot{q_i} + \boldsymbol{v^R_{i}}\times \boldsymbol{s_i}G_i\dot{q_i}$ 
    \State $\boldsymbol{f^R_i = I^R_{i}a^R_{i} + S(v^R_{i})I^R_{i}v^R_{i}}$
\EndFor

\For{$i=N_B$ to $1$}
    \State $\tau_{gear_i} = \boldsymbol{s_i^Tf_i}$
    \State $\tau_{friction_i} = b^s_isign(\dot{q_i}) + b^v_i(\dot{q_i})$
    \State $\tau_{motor_i} = \tau_{gear_i}/G_i + \boldsymbol{s_i^Tf^R_i} + \tau_{friction_i}$
\If{$\lambda(i) \neq 0$}
    \State $\boldsymbol{f_{\lambda(i)} = f_{\lambda(i)} +{}^{\lambda(i)}X^*_if_i + {}^{\lambda(i)}X^*_if^R_i}$
\Else
    \State $\boldsymbol{\tau_{v} = f_{v} + {}^{v}X^*_1f_1 + {}^{v}X^*_1f^R_1 }$
\EndIf
\EndFor

\end{algorithmic}
\end{algorithm}
%\vspace{-4pt}

%
The process follows a two-pass structure. In the first pass, the body forces, velocities, and accelerations are  propagated from the  free-floating base to the end-effector of the manipulator. For each link \(i\) with $i \in  \{1, .., N_B\}$, where $N_B$ is the number of bodies in the kinematic chain, the joint model describes the transformation matrix \( \boldsymbol{{}^{i}X_{\lambda(i)}}\) between consecutive links and the corresponding axis of rotation presented as a vector, \(\boldsymbol{s_i}\). The transformation from the first link of the manipulator to the free-floating base is computed using line $4$ in Algorithm~\ref{alg:hyd_rnea}. In this algorithm body $0$ is the first link of the manipulator attached to the free-floating base. 
%
%If the link is not directly connected to body 0 (\(\lambda(i) \neq 0\)), its transformation relative to the base, \(\boldsymbol{{}^iX_{\lambda(i)}{}^{\lambda(i)}X_0{}^0X_{base}} \), is computed. This is used in modeling the restoring forces of the system.
%
Body 0's linear and angular velocity, \(\boldsymbol{v_0}\) and its acceleration, \(\boldsymbol{a_0}\) are initialized to the velocity and acceleration projected from the base vehicle (lines $6$ and $7$ in Algorithm~\ref{alg:hyd_rnea}). The subsequent manipulator links velocities \(\boldsymbol{v_i}\) and accelerations \(\boldsymbol{a_i}\) are calculated recursively using the transformation between consecutive links  \(\boldsymbol{{}^{i}X_{\lambda(i)}}\) and projected joint velocities/accelerations \(\dot{q}^n_i\) and \(\ddot{q}^n_i\). In line $11$ of Algorithm $1$, the forces \(\boldsymbol{f_i}\) acting on the link due to the rigid body forces (line $14$, where $S(\cdot)$ is the cross-product operator) and hydrodynamic forces $\boldsymbol{f_i^H}$ are computed. Lines $15$ to $17$ describe the joint rotor dynamics, where $G_i$ is the gear ratio at joint $i$, $\boldsymbol{I^R_i}$ the rotor inertia,  $\boldsymbol{a_i^R}$  and $\boldsymbol{v_i^R}$ are the rotor's acceleration and velocity. To the best of our knowledge, it is the first time that the rotor dynamics have been included in the Recursive Newton-Euler formulation.

In the second pass, data propagates from the end-effector to the free-floating base. For each link the joint torque \(\tau_{gear_i}\) is computed by projecting the link forces \(\boldsymbol{f_i}\) onto the joint axis \(s_i\). Friction $\tau_{friction_i}$ is calculated by considering static and dynamic friction components (\(b^s_i\) and \(b^v_i\)). The motor torque \(\tau_{motor_i}\) required to overcome the friction and produce the resulting joint motion is computed in line $22$. Next the forces are propagated back as \(\boldsymbol{f_{\lambda(i)}}\) and \(\tau_{motor_{\lambda(i)}}\) calculations repeat. In the case of the free-floating base, the total forces and moments \(\boldsymbol{\tau_{base}}\) are computed by summing projected forces and moments from the first link of the manipulator  and the corresponding rotor, in addition to the bases' initially forces and moment.
